# Supplementary material for: Toward Large Kernel Models
Source: arXiv:2302.02605 source file (2023-06-20)
Supplement: Supplementary file 1 [file proof_convergence.tex]

\begin{proof}[Proof of \Cref{lem:projection}]
\begin{align}
    \text{proj}_{\mathbb{Z}}\curly{f^t-\eta\mc  P\curly{g}^t}
    &=K(\cdot,Z)K(Z,Z)\inv\round{f^t(Z)-\eta\,\mc P\curly{g}^t(Z)}\\
    &=K(\cdot,Z)K(Z,Z)\inv\round{K(Z,Z)\alphavec^t-\eta\,\mc P\curly{g}^t(Z)}\\
    &=K(\cdot,Z)\alphavec^t-\eta\,K(\cdot,Z)K(Z,Z)\inv\round{\mc P\curly{g}^t(Z)}\\
    &= f^t - \eta\,K(\cdot,Z)K(Z,Z)\inv\round{\mc P\curly{g^t}(Z)}
\end{align}
\end{proof}

\begin{align*}
    \alphavec^{t+1}=\alphavec^t-\eta_t\Pi (K(X,Z)\tran-K(X,Z)\tran EDE\tran K(X,X))\g^t\\
    \alphavec^{t+1}=\alphavec^t-\eta_t\Pi (K(X,Z)\tran-K(X,Z)\tran e_1(1-\tfrac{\lambda_{2}}{\lambda_1}) e_1\tran)\g^t
\end{align*}
where $\g^t=K(X,Z)\alphavec^t-\y$. 
At convergence, this means
\begin{align}
    K(X,Z)\tran(I_n-(1-\tfrac{\lambda_2}{\lambda_1})e_1e_1\tran)K(X,Z)\alphavec=K(X,Z)\tran(I_n-(1-\tfrac{\lambda_2}{\lambda_1})e_1e_1\tran)\y
\end{align}

For ease of notation below, we refer to $K(X,Z)=XZ\tran$ with $X,Z$ full row-rank matrices with $n$ and $p$ rows respectively. Let $a=1-\frac{\lambda_2}{\lambda_1}$. Thus the fixed point satisfies
\begin{align}
    ZX\tran(I_n - a e_1e_1\tran)(XZ\tran\alpha-y)=0
\end{align}
Let $X=E\Lambda^{.5}F\tran$ with $E\tran E=EE\tran=I_n$, and $\alpha_2$ be the solution. Then we have
\begin{align}
    ZF\Lambda^{.5}E\tran(I_n - a e_1e_1\tran)(E\Lambda^{.5}F\tran Z\tran\alpha_2-y)&=0\\
    ZF\Lambda^{.5}(I_n - a e_1e_1\tran)(\Lambda^{.5}F\tran Z\tran\alpha_2-E\tran y)&=0\\
    H\tran \Lambda^{.5}(I_n-E_q(I_q-\lambda_{q+1}\Lambda_{q}\inv) E_q\tran)\Lambda^{.5}(H\alpha_2-G y)&=0\\
    H\tran D(H\alpha_2-G y)&=0\qquad D=\Lambda-J\\
    \alpha_2 = (H\tran D H)\inv H\tran D Gy
    % H\tran \Lambda(H\alpha_2 - Gy)&=H\tran J(H\alpha_2-Gy)
\end{align}
where $H\tran=ZF$ and $G=\Lambda^{-.5}E\tran$, and $J=\Lambda^{.5} E_q(I_q-\lambda_{q+1}\Lambda_q\inv)E_q\tran\Lambda^{.5}$. Whereas the OLS solution $\alpha_1$ satisfies
\begin{align}
    ZX\tran (XZ\tran\alpha_1-y)&=0\\
    ZF\Lambda^{.5}E\tran (E\Lambda^{.5}F\tran Z\tran\alpha_1-y)&=0\\
    H\tran \Lambda(H\alpha_1 - Gy)&=0\\
    \alpha_1 = (H\tran\Lambda H)\inv H\tran \Lambda Gy
\end{align}
Let us calculate the least squares loss of both solutions. Note $\norm{XZ\tran\alpha-y}^2=\norm{E\Lambda^{.5}H\alpha-y}^2=\norm{\Lambda^{.5}\round{H\alpha-Gy}}^2$. 
\begin{align}
    \norm{\Lambda^{.5}\round{H\alpha_1-Gy}}^2&=y\tran G\tran\Lambda Gy-y\tran G\tran\Lambda H\alpha_1+\alpha_1\tran H\tran\Lambda(H\alpha_1-Gy)\\
    &=\norm{y}^2-y\tran G\tran\Lambda H\alpha_1
\end{align}
\begin{align}
    \norm{\Lambda^{.5}\round{H\alpha_2-Gy}}^2 &= \norm{y}^2 - y\tran G\tran\Lambda H\alpha_2 + \alpha_2\tran H\tran\Lambda (H\alpha_2-Gy)\\
    &= \norm{y}^2 - y\tran G\tran\Lambda H\alpha_2 + \alpha_2\tran H\tran J (H\alpha_2-Gy)\\
    &= \norm{y}^2 - y\tran G\tran(\Lambda+J) H\alpha_2 + \alpha_2\tran H\tran J H\alpha_2
\end{align}
