# Supplementary material for: Toward Large Kernel Models
Source: arXiv:2302.02605 source file (2023-06-20)
Supplement: Supplementary file 2 [file proof_generalization.tex]

Note that $GG\tran=\Lambda\inv$, and $G\tran G=XX\tran$
Assuming a student-teacher model, with
\begin{align}
    y &= K(X, Z) \alpha^* + \xi\\
    y &= G\tran \Lambda H \alpha^* + \xi\\
    \alpha_1 &= (H\tran\Lambda H)\inv H\tran \Lambda Gy=(H\tran\Lambda H)\inv H\tran \Lambda GG\tran\Lambda H\alpha^* + (H\tran\Lambda H)\inv H\tran \Lambda G\xi\\
    &=\alpha^*+(H\tran\Lambda H)\inv H\tran \Lambda G\xi\\
    \alpha_2 &= (H\tran D H)\inv H\tran D Gy=(H\tran D H)\inv H\tran D GG\tran\Lambda H\alpha^* + (H\tran D H)\inv H\tran D G\xi\\
    &=\alpha^* + (H\tran D H)\inv H\tran D G\xi
\end{align}

Now, assuming gaussian noise, $\xi\sim\mc N(0, \I_n),$ we have
\begin{align}
    \Exp\norm{f_1-f^*}_{L^2_{\mathbb{P}_X}}^2 &= \Exp\norm{K(X, Z)(\alpha_1-\alpha^*)}^2=\Exp\norm{G\tran \Lambda H(H\tran\Lambda H)\inv H\tran \Lambda G\xi}^2\\
    &=\frac{\sigma^2}n\trace\round{G\tran\Lambda H(H\tran\Lambda H)\inv H\tran \Lambda GG\tran \Lambda H(H\tran\Lambda H)\inv H\tran \Lambda G}\\
    &=\frac{\sigma^2}n\trace\round{\I_p}=\sigma^2 p/n
\end{align}
and similarly,
\begin{align}
    \Exp\norm{f_2-f^*}_{L^2_{\mathbb{P}_X}}^2 &= \Exp\norm{K(X, Z)(\alpha_2-\alpha^*)}^2=\Exp\norm{G\tran \Lambda H(H\tran D H)\inv H\tran D G\xi}^2\\
    &=\trace\round{G\tran D H(H\tran D H)\inv H\tran \Lambda GG\tran\Lambda H(H\tran D H)\inv H\tran D G}\\
    &=\trace\round{H\tran D\Lambda\inv DH(H\tran D H)\inv H\tran \Lambda H(H\tran D H)\inv}
\end{align}
\subsection{Convergence}
Consider a linear dynamical system
\begin{align}
    \x^{t} 
    &= \A\x^{t-1} + \b\\
    &= \A^t \x_0 + \sum_{i=0}^{t-1} \A^i b
\end{align}
Solving $K(Z,Z)\thetavec=\h$ with a preconditioned Richardson update for $T$ steps from $\zero_p$ gives,
\begin{align}
    \thetavec^{+} &= \thetavec - \nu(\I_p-\Q_2)(K(Z, Z) \thetavec - \h)
       = (\I_p - \nu(\I_p-\Q_2)K(Z, Z)) \thetavec + \nu(\I_p-\Q_2) \h\\
\thetavec^T &= \nu \sum_{i=0}^{T-1} (\I_p-\nu (\I_p-\Q_2) K(Z, Z))^i (\I_p-\Q_2) \h
\end{align}

For $\h=K(Z,X)(\I_n-\Q_1)(K(X,Z)\alphavec-\y)$, we get
\begin{align*}
    \alphavec^+ 
    &= \alphavec - \eta \theta^T\\
    &= \alphavec - \eta \nu \sum_{i=0}^{T-1} (\I_p-\nu (\I-\Q_2) K(Z, Z))^i (\I_p-\Q_2) K(Z,X)(\I_n-\Q_1)(K(X,Z)\alphavec-\y)\\
    &= (\I_p - \eta \nu \A K(X,Z)) \alphavec + \A \y
\end{align*}
where 
\begin{align}
    \A=\sum_{i=0}^{T-1} (\I_p-\nu (\I_p-\Q_2) K(Z, Z))^{i} (\I_p-\Q_2) K(Z,X)(\I_n-\Q_1)
\end{align}

The convergence of this depends on the spectrum of
\begin{align}
    \norm{\A K(X,Z)}
    &\leq \sum_{i=0}^{T=1}\norm{(\I_p-\nu (\I_p-\Q_2) K(Z, Z))^{i} (\I_p-\Q_2) K(Z,X)(\I_n-\Q_1)K(X,Z)}\\
    &\leq \sum_{i=0}^{T-1} (1-\nu(\lambda_1-\lambda_{\xi+1}))^i \frac{1}{\lambda_{q+1}}\sigma_{\rm max}^2(K(X,Z))
\end{align}
