# Supplementary material for: Toward Large Kernel Models
Source: arXiv:2302.02605 source file (2023-06-20)
Supplement: Supplementary file 3 [file convergence.tex]

\subsection{Convergence analysis: Variance reduction due to data preconditioning}

For the purpose of convergence, we focus on EigenPro\,3.0, the simplest iteration without any optimizations from EigenPro\,3.1.
Define $\bm{P}:=\I_n-\Q_n$.
\begin{lemma}
Algorithm \ref{alg:eigenpro30}, with $s=m=n,$ to $\sigma=p$ converges if $\eta<\frac{2}{\lambda_{q+1}}$ and
\begin{align}
    \alphavec^\infty &= 
    \big(K(Z,X)\bm{P}K(X,Z)\big)\inv K(Z,X)\bm{P}\y\\
    \alphavec^T &= 
    (I_p-\sum_{i=1}^{T-1} \eta^i\big(K(Z,Z)\inv K(Z,X)\bm{P}K(X,Z)\big)^i K(Z,X)\bm{P})(K(X,Z)\alpha^0-\y)\\
\end{align}
Furthermore,
\begin{align}
    \norm{\alphavec^T-\alpha^\infty}&\leq \round{1-\frac{\nu\eta}{\kappa}}^T
\end{align}
\end{lemma}
